# Supplementary material for: Transport and information in open quantum systems
Source: arXiv:2401.13292 source file (2024-01-24)
Supplement: Supplementary file 1 [file Appendix.tex]

\setcounter{equation}{0}
Here we will carry out the integral in \eqref{eq:MeasurementsP1} for the probability to obtain a single A detection event. By inserting the expressions of \eqref{eq:MeasurementsEoMGround} and \eqref{eq:MeasurementsEoMExcited}, we find that
\begin{align}
P_\text{A}
=& \int_0^\infty\mathrm{d}t\, \mu\Gamma \frac{\rho_{ee}{}^2(t)}{\rho_{gg}(t)} \nonumber\\
=& \mu \Gamma \int_0^\infty\mathrm{d}t\, \frac{\pi_e{}^2\,\exp\left(\frac{-2\mu}{1-\mu}\frac{\pi_e}{\pi_g}\right) \exp(-2\Gamma t) \exp\left(\frac{2\mu}{1-\mu}\frac{\pi_e}{\pi_g} \exp(-\Gamma t)\right)}{\pi_g \exp\left(\frac{-\mu}{1-\mu}\frac{\pi_e}{\pi_g}\right) \exp\left(\frac{\mu}{1-\mu}\frac{\pi_e}{\pi_g}\right)} \nonumber\\
=& \mu \Gamma \frac{\pi_e{}^2}{\pi_g} \exp\left(\frac{-\mu}{1-\mu}\frac{\pi_e}{\pi_g}\right) \int_0^\infty\mathrm{d}t\, \exp(-2\Gamma t)  \exp\left(\frac{\mu}{1-\mu}\frac{\pi_e}{\pi_g}\exp(-\Gamma t)\right)\nonumber \\
=& \frac{\mu \pi_e{}^2}{\pi_g}\, \left(\frac{\exp\big(A\big)}{A^2} + \frac{1-\exp\left(A\right)}{A^3}\right),
\label{eq:AppendixAP_A}
\end{align}
where we have defined 
\begin{equation}
A = \exp\left(\frac{\mu}{1-\mu}\frac{\pi_e}{\pi_g}\right).
\end{equation}

In the same manner as above we may determine the probability of a B detection event followed by an A detection event, $P_\text{BA}$. This involves an integral over the corresponding two times $t_B$ and $t$ for respectively the B-jump and the A-jump. Letting $\rho_{B,ee}(t)$ and $\rho_{B,gg}(t)$ denote density matrix elements evolved to the time $t$ conditioned on the outcome of the B-jump at time $t_B$ as given by \eqref{eq:MeasurementsBJumpState}, we find that
\begin{align}
P_\text{BA} =& \int_0^\infty\text{d}t\,  \mu\Gamma \frac{\rho_{B,ee}{}^2(t)}{\rho_{B,gg}(t)} \int_0^t\text{d}t_\text{B}\, \frac{\Gamma}{1-\mu}\rho_{ee}(t_\text{B})\left(1+\mu^2 \frac{\rho_{ee}(t_\text{B})}{\rho_{gg}(t_\text{B})}\right)\nonumber\\
=& A_0 \int_0^\infty\text{d}t\, \Gamma\exp(-2 \Gamma t) \exp\Big(A_2\, \exp(-\Gamma t)\Big) 
\nonumber\\
&\times\int_0^t\text{d}t_\text{B}\,\Gamma\exp(-\Gamma t_\text{B}) \exp\Big(A_1\,\exp(-\Gamma t_\text{B})\Big)\nonumber \\
=& \frac{A_0}{A_1}\bigg\{\exp(A_2)\left[\frac{1-\exp(A_2)}{A_2^2} + \frac{\exp(A_2)}{A_2} \right] \nonumber\\
& - \left[\frac{1 - \exp(A_1+A_2)}{(A_1+A_2)^2} +\frac{\exp(A_1+A_2)}{A_1+A_2}\right]\bigg\},
\label{eq:AppendixAP_BA}
\end{align}
where we have defined
\begin{align}
A_0 =& \frac{\mu^5}{1-\mu}\frac{\pi_e^3}{\pi_g^2}\exp\left(\frac{-\mu}{1-\mu}\frac{\pi_e}{\pi_g}\right), \nonumber\\
A_1 =& (\mu+\mu^2)\frac{\pi_e}{\pi_g}, \\
A_2 =& \frac{\mu^3}{1-\mu}\frac{\pi_e}{\pi_g}. \nonumber
\end{align}
